# Supplementary material for: Neural Temporal Point Processes For Modelling Electronic Health Records
Source: arXiv:2007.13794 source file (2020-12-07)
Supplement: Supplementary file 1 [file language-model.tex]

\section{Temporal Point Processes as a language model}
The standard $n$-gram language model is given by:
\begin{equation}
    p(\{x_1,x_2,\ldots,x_N\})=\prod_{i=1}^Np(x_i|\{x_j|j<i\})
\end{equation}
Now imagine that each of the $x_i$ are actually binned ``bags'' of representations within a time interval $[t_i,t_i+\Delta t)$, and if we're considering multi-class learning, we allow a ``nothing happened here`` token, \texttt{<NONE>}.
Then a sequence might look like, for some sampling granularity $\Delta t$

$1.2(0.1)$

\begin{equation}
    \texttt{<START>},\texttt{<NONE>},\texttt{<NONE>},\texttt{<THING>},\texttt{<NONE>},\ldots
\end{equation}
A \gls{tpp} is, roughly speaking, a language model where 
$\Delta t\rightarrow0$, and instead of having explicit \texttt{<NONE>} tokens, gaps between events are treated analytically as a continuum of \texttt{<NONE>} tokens by the conditional density $p_m(t|\mcH_t)$.
